# Supplementary material for: Short-reach Optical Communications: A Real-world Task for Neuromorphic Hardware
Source: arXiv:2412.03129 source file (2024-12-04)
Supplement: Supplementary file 1 [file appendix.tex]

\section{Appendix}
